# Supplementary material for: Critical field anisotropy in the antiferroelectric switching of PbZrO3 films
Source: arXiv:2009.06561 ancillary file (2020-12-21)
Supplement: Supplementary file 1 [file Supplemental_Information.pdf]

# Critical field anisotropy in the antiferroelectric switching of $\text{PbZrO}_3$ films - Supplemental information

Cosme Milesi-Brault,<sup>1,2,3,\*</sup> Nicolas Godard,<sup>1,2,3</sup> Stéphanie Girod,<sup>1,3</sup> Yves Fleming,<sup>1</sup> Brahime El Adib,<sup>1</sup> Nathalie Valle,<sup>1</sup> Sebastjan Glinšek,<sup>1,3</sup> Emmanuel Defay,<sup>1,3</sup> and Mael Guennou<sup>2,3,†</sup>

<sup>1</sup>*Materials Research and Technology Department,*

*Luxembourg Institute of Science and Technology, 41 rue du Brill, L-4422 Belvaux, Luxembourg.*

<sup>2</sup>*Department of Physics and Materials Science, University of Luxembourg, 41 rue du Brill, L-4422 Belvaux, Luxembourg.*

<sup>3</sup>*Inter-institutional Research Group Uni.lu-LIST on ferroic materials, 41 rue du Brill, L-4422 Belvaux, Luxembourg*

## CONTENTS

|                                                      |   |
|------------------------------------------------------|---|
| I. Details of the deposition parameters              | 2 |
| II. SEM: surface, cross-section and grain size       | 3 |
| III. Secondary Ion Mass Spectrometry (SIMS) analysis | 4 |
| IV. Pole figures                                     | 5 |
| V. Evidence of tensile strain by XRD measurements    | 6 |
| VI. Frequency dependence of the double loops         | 7 |
| VII. Compilation of literature data                  | 8 |
| References                                           | 9 |

---

\* cosme.milesi@list.lu

† mael.guennou@uni.lu

## I. DETAILS OF THE DEPOSITION PARAMETERS

Lead zirconate ( $\text{PbZrO}_3$ ) films were deposited by chemical solution deposition (CSD) on two different substrates: platinized silicon ( $\text{Si}/\text{SiO}_2$  500 nm/ $\text{TiO}_x$  20 nm/ $\text{Pt}$  100 nm) and fused silica covered with a 23 nm-thick ALD-deposited  $\text{HfO}_2$  buffer layer. In both cases, a seed layer of lead titanate ( $\text{PbTiO}_3$ ) was deposited prior to  $\text{PbZrO}_3$ .

Lead zirconate solutions were processed following a standard process based on mixing freeze-dried lead(II) acetate trihydrate (99.9%, Sigma-Aldrich, USA) and zirconium(IV) propoxide (70% in propanol, Sigma-Aldrich, USA) into anhydrous 2-methoxyethanol (2-ME, Sigma-Aldrich, USA). Prior mixing the zirconium precursor was modified using two equivalents of acetylacetone (99.5%, Sigma-Aldrich, USA). Due to lead volatility, an excess of 20% of lead is added to the solution to target a stoichiometric ratio of lead and zirconium in the crystallised films. This solution was then refluxed, distilled and diluted to reach a concentration of 0.3 M. A similar process was used to prepare the 0.1 M  $\text{PbTiO}_3$  solution, with acetylacetone-modified titanium(IV) isopropoxide (97%, Sigma-Aldrich, USA) used as a titanium precursor and with 30% excess of lead. Two solutions of  $\text{PbTiO}_3$  were prepared using 2-ME and 1-methoxy 2-propanol (1M-2P) as solvents, in order to modify the degree of preferred orientation, as reported in [1].

Films were then obtained by spin-coating the  $\text{PbZrO}_3$  solution on top of this seed layer, drying it at 130 °C for 3 minutes and pyrolyzing at 350 °C for 3 minutes. These three steps were repeated to increase the thickness of the samples. The final crystallization was done by a rapid thermal annealing of the stack at 700 °C in an Annealsys AS-Master rapid thermal annealing furnace for 5 minutes. Films with thicknesses of 85 nm, 170 nm and 255 nm were obtained.

On platinized silicon, 100 nm-thick circular Pt electrodes were sputtered. On fused silica, Pt interdigitated electrodes (IDE) with a gap of 5  $\mu\text{m}$  were sputtered and patterned with lift-off photolithography.

## II. SEM: SURFACE, CROSS-SECTION AND GRAIN SIZE

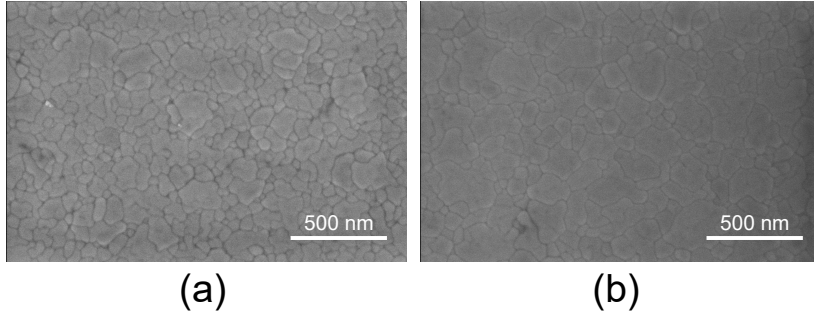

Figure S1: SEM surface micrographs of (a) 85 nm-thick and (b) 170 nm  $\text{PbZrO}_3$  samples in a MIM "high orientation" geometry

Average grain size have been estimated by the intercept method for these two micrographs: around  $86 \pm 9$  nm for the 85 nm-thick film and around  $112 \pm 13$  nm for the 170 nm-thick.

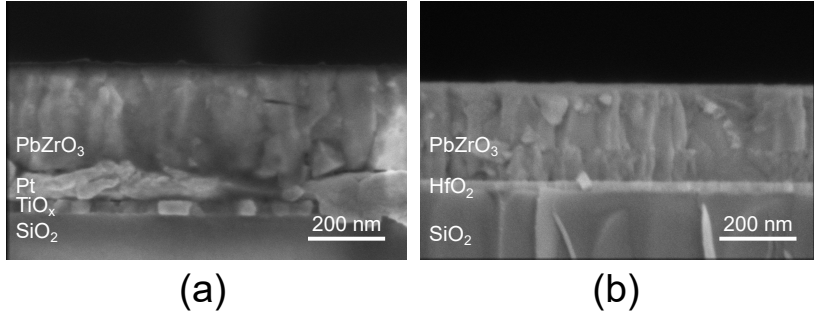

Figure S2: SEM cross-section micrographs of 255 nm-thick  $\text{PbZrO}_3$  in (a) MIM "highly oriented" geometry and (b) IDE geometry

These cross-sections highlight the columnar microstructure of our  $\text{PbZrO}_3$  films in both geometries. Moreover, we observe that the width of these columnar grains is quite similar between both geometries.

### III. SECONDARY ION MASS SPECTROMETRY (SIMS) ANALYSIS

Secondary Ion Mass Spectrometry (SIMS) depth profiles have been performed to verify the composition of the films through the thickness. These experiments were performed on a CAMECA C-Ultra. Primary bombardment of  $\text{Cs}^+$  ions at 1 keV was used to analyze an area of  $60\text{ }\mu\text{m}$  in diameter over a  $250\text{ }\mu\text{m} \times 250\text{ }\mu\text{m}$  rastered area.

The SIMS ratio of Pb/Zr evolves similarly in both samples (Fig.3 a.), showing no noticeable difference between the two different geometries. The small dips can be traced back to the preparation method and the two annealing steps performed for the deposition of thicker films. Fig. 3(b) shows the raw SIMS intensity for Ti. The more intense peak shows the location of the  $\text{PbTiO}_3$  seed layer. For the MIM sample, a secondary peak is observed on the left, indicating that some diffusion of Ti has occurred over a small thickness in the  $\text{PbZrO}_3$  layer. The integrated Ti signal is nearly identical between the two samples, which indicates that Ti diffusion from the  $\text{TiO}_x$  layer across the Pt electrode in the MIM sample, if it occurs, remains limited.

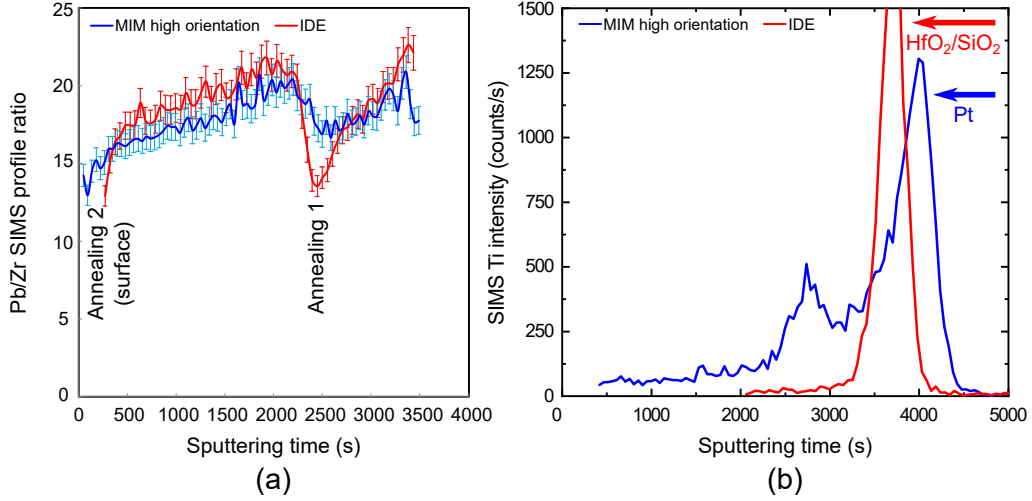

Figure S3: SIMS depth profiles for samples in both the MIM and the IDE geometry. The zero position on the  $x$ -axis corresponds to the film top surface, and the thickness is measured by the sputtering time. (a) Ratio of Zr/Pb SIMS signals through the film thickness. The ratio of SIMS signal is proportional but not equal to the true composition ratio. (b) Evolution of Ti SIMS intensities through the  $\text{PbZrO}_3$  layer up to the interface with the Pt layer (in MIM geometry) or the  $\text{SiO}_2$

## IV. POLE FIGURES

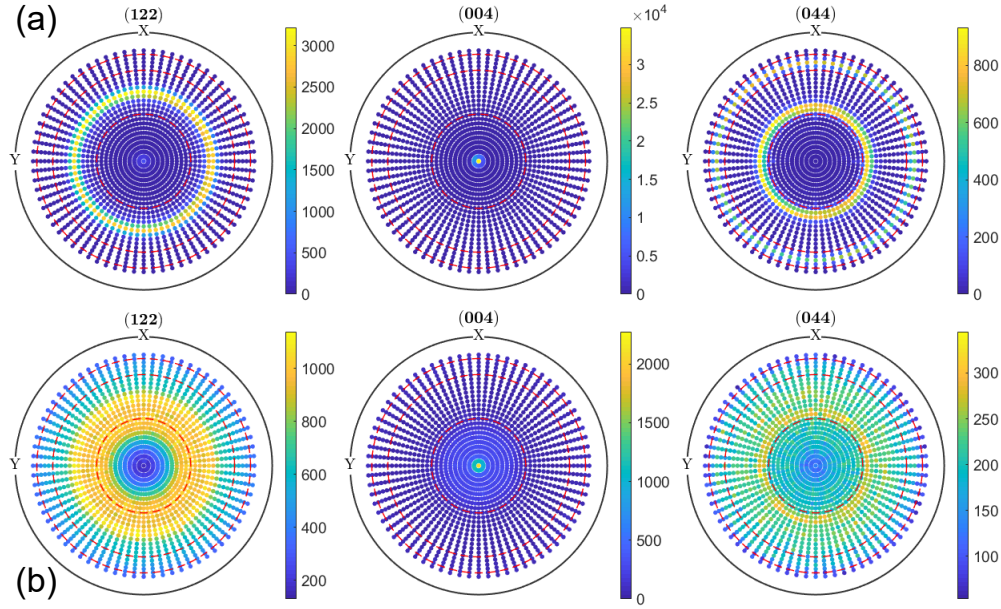

Figure S4: Pole figures of a 255 nm-thick  $\text{PbZrO}_3$  samples in (a) MIM "high orientation" geometry and (b) IDE geometry

The pole  $(004)_o$  confirms the very high orientation of the MIM film and the slightly lower-oriented IDE film. The high intensity rings around the center of poles  $(122)_o$  and  $(044)_o$  prove that the diffraction intensity at these poles is invariant with the rotation of the film in plane. Hence, these pole figures confirm the isotropic in-plane orientation of the  $\text{PbZrO}_3$  films in both geometries. The higher width of these rings can be directly linked to the lower orientation of the IDE film compared to the MIM high orientation.

These pole figures have not been corrected from the potential defocalization happening during these long scans.

## V. EVIDENCE OF TENSILE STRAIN BY XRD MEASUREMENTS

Stresses and strains are expected in polycrystalline films due to a mismatch in the thermal expansion coefficient (TEC) between the substrate and the deposited material. Here, we use silicon ( $2.6 \times 10^{-6} \text{ K}^{-1}$ ) and fused silica ( $5.5 \times 10^{-7} \text{ K}^{-1}$ ). In both cases, this mismatch is expected to drive the  $\text{PbZrO}_3$  films in a tensile strain state, as the TEC of  $\text{PbZrO}_3$  is much higher, around  $8.0 \times 10^{-6} \text{ K}^{-1}$  [2].

XRD measurements were performed to estimate the strain state of our films, following the procedure described in Schenk et. al. [3]. For this analysis, the  $(111)_{\text{pc}}$  reflection was recorded at several values of the angle  $\Psi$ , obtained by rotating the sample so as to tilt the scattering vector away from the sample normal (Fig. 5(a)). This peak was chosen because it does not split in the orthorhombic structure expected for PZO. Following this approach, the sign of the slope of the interplanar distance  $d_{(111)}(\Psi)$  with respect to  $\sin^2 \Psi$  reflects the sign of the in-plane strain  $\varepsilon$ . If the position of the  $(111)_{\text{pc}}$  peak shifts towards lower values when  $|\Psi|$  increases, then the strain is positive and the film is in a tensile state. The opposite holds for a compressive state.

The figure below shows the  $(111)_{\text{pc}}$  reflection as a function of  $\Psi$  for films on both Pt/Si and fused silica. Due to the high film texturation, the peak is visible only in a limited angular range. We observe that it shifts towards lower  $2\theta$  values with increasing  $\Psi$  values, confirming that the films experience tensile strain in both cases. On the other hand, a quantitative estimation of the strain values is here not possible because this measurement alone does not allow us to disentangle the contributions of the orthorhombic spontaneous strains and of the residual strain.

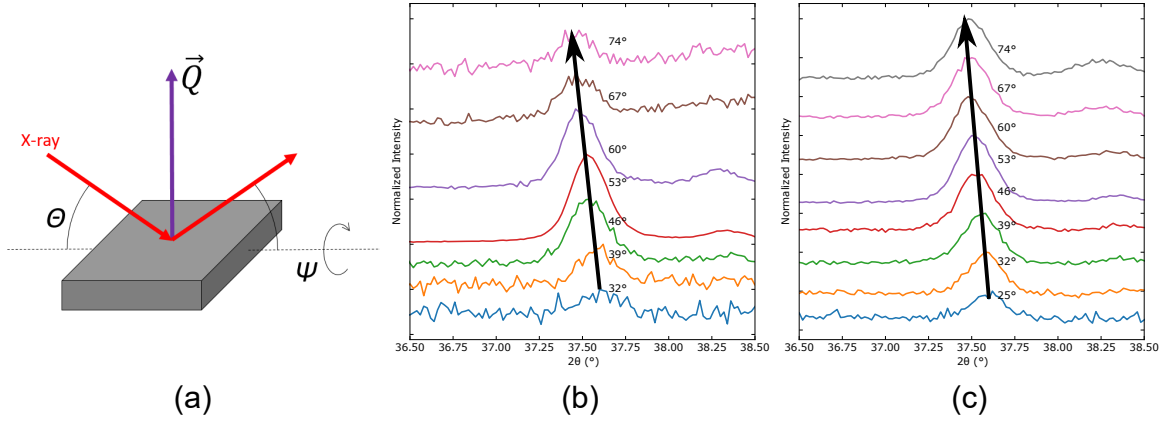

Figure S5: (a) Sketch of the diffraction geometry used to estimate the strain state of our films.  $\theta - 2\theta$  scans of the  $(111)_{\text{pc}}$  reflection at several values of  $\Psi$  for a 255 nm-thick sample in (b) MIM and (c) IDE geometry. Black arrows highlight the shift of the position of the  $(111)_{\text{pc}}$  peak

## VI. FREQUENCY DEPENDENCE OF THE DOUBLE LOOPS

The  $P(E)$  loops reported in the main paper were measured at 100 Hz. The frequency dependence of the loops was checked and a double loop was observed in all cases, whereby the fields show a weak frequency dependence. In Fig. S6, we show the frequency dependence of the switching fields between 10 Hz and 5 kHz for a representative 255 nm-thick MIM sample. The values are found to vary within 5.5% of the average value. This is less than the error bars of 10% reported in Fig. 4 in the main paper. Capacitance measurements have been performed on 255 nm-thick MIM samples, with high and low  $(001)_{\text{pc}}$  orientation (Fig. S7). Texture doesn't seem to influence strongly the dielectric constant of the material, neither does the measurement frequency.

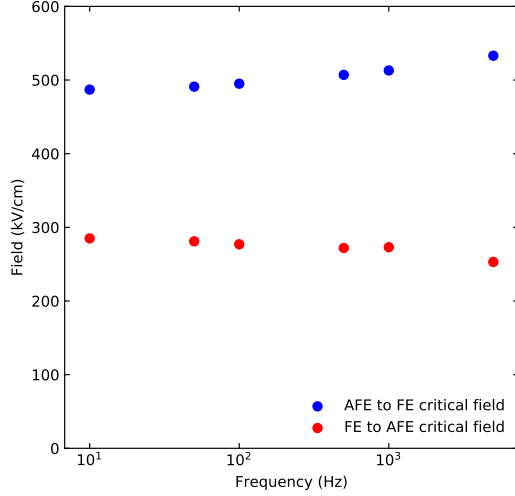

Figure S6: Frequency dependence of the critical fields ( $E_{\text{AFE} \rightarrow \text{FE}}$  and  $E_{\text{FE} \rightarrow \text{AFE}}$ ) on a 255 nm-thick highly oriented MIM sample

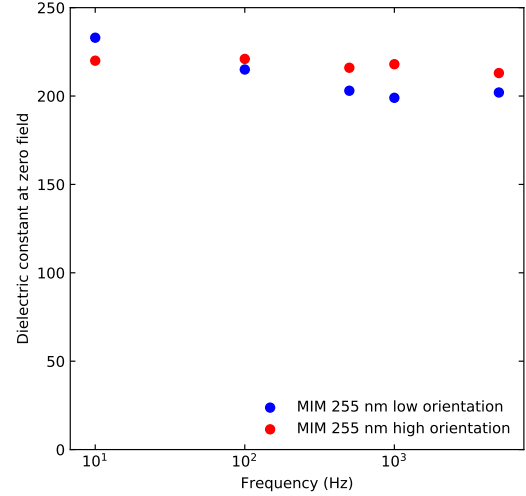

Figure S7: Frequency dependence of dielectric constant on 255 nm-thick low and high orientation MIM samples

## VII. COMPILATION OF LITERATURE DATA

Table S1: Review of papers reporting antiferroelectric switching of undoped  $\text{PbZrO}_3$ . Unless stated otherwise, measurements have been conducted at room temperature and with an out-of-plane field, in a MIM geometry.

| Processing method                    | Thickness       | $E_{\text{AFE} \rightarrow \text{FE}}$<br>(kV/cm) | $E_{\text{FE} \rightarrow \text{AFE}}$<br>(kV/cm) | $P_s$<br>( $\mu\text{C}/\text{cm}^2$ ) | Orientation                     | Substrate (bottom $\rightarrow$ top)                                   | Reference     |
|--------------------------------------|-----------------|---------------------------------------------------|---------------------------------------------------|----------------------------------------|---------------------------------|------------------------------------------------------------------------|---------------|
| Sol-gel                              | 85 nm           | 501                                               | 239                                               | 25.3                                   | (002) <sub>o</sub>              | Si/SiO <sub>2</sub> /TiO <sub>x</sub> /Pt                              | This work MIM |
|                                      | 170 nm          | 425                                               | 233                                               | 22.3                                   | (002) <sub>o</sub>              | Si/SiO <sub>2</sub> /TiO <sub>x</sub> /Pt                              | This work MIM |
|                                      | <b>255 nm</b>   | <b>495</b>                                        | <b>296</b>                                        | <b>24.4</b>                            | (002) <sub>o</sub>              | Si/SiO <sub>2</sub> /TiO <sub>x</sub> /Pt                              | This work MIM |
|                                      | 85 nm           | 219                                               | 95                                                | 21.9                                   | (002) <sub>o</sub>              | SiO <sub>2</sub> /HfO <sub>2</sub>                                     | This work IDE |
|                                      | 170 nm          | 333                                               | 170                                               | 35.8                                   | (002) <sub>o</sub>              | SiO <sub>2</sub> /HfO <sub>2</sub>                                     | This work IDE |
|                                      | <b>255 nm</b>   | <b>286</b>                                        | <b>134</b>                                        | <b>17.7</b>                            | (002) <sub>o</sub>              | SiO <sub>2</sub> /HfO <sub>2</sub>                                     | This work IDE |
|                                      | 120 nm          | 162                                               | -                                                 | 20                                     | (111) <sub>pc</sub>             | Si/SiO <sub>2</sub> /TiPt                                              | [4]           |
|                                      | 500 nm          | 350                                               | 260                                               | 25                                     | (111) <sub>pc</sub>             | "Pt-buffered silicon"                                                  | [5]           |
|                                      | 496 nm          | 430                                               | 300                                               | 25                                     | (111) <sub>pc</sub>             | Si/SiO <sub>2</sub> /Ti/Pt                                             | [6]           |
|                                      | 500 nm          | 460                                               | 250                                               | 30                                     | (111) <sub>pc</sub>             | Si/SiO <sub>2</sub> /Ti/Pt                                             | [7]           |
|                                      | -               | 250                                               | 125                                               | -                                      | (100) <sub>pc</sub>             | Si/SiO <sub>2</sub> /Ti/Pt                                             | [8]           |
|                                      | 450 nm          | 450                                               | -                                                 | 20                                     | (100) <sub>pc</sub>             | Si/SiO <sub>2</sub> /Ti/Pt/LaNiO <sub>3</sub>                          | [9]           |
|                                      | 900 nm          | 700                                               | -                                                 | 20                                     | (100) <sub>pc</sub>             | Si/SiO <sub>2</sub> /Ti/Pt/LaNiO <sub>3</sub>                          | [9]           |
|                                      | 248 nm          | 491                                               | 193                                               | 25                                     | (100) <sub>pc</sub>             | Si/SiO <sub>2</sub> /Ti/Pt                                             | [10]          |
|                                      | 575 nm          | 460                                               | 200                                               | 39                                     | (001) <sub>pc</sub>             | Si/SiO <sub>2</sub> /Ti/Pt                                             | [11]          |
|                                      | 900 nm          | 500                                               | 230                                               | 40                                     | (001) <sub>pc</sub>             | Si/SiO <sub>2</sub> /Ti/Pt/LaNiO <sub>3</sub>                          | [12]          |
|                                      | 650 nm          | 250                                               | -                                                 | 24                                     | -                               | "Pt/Ti-coated silicon"                                                 | [13]          |
|                                      | 800 nm          | 400                                               | 200                                               | 34                                     | Mixed orientation               | "Pt/Ti-coated silicon" + TiO <sub>2</sub>                              | [14]          |
|                                      | 650 nm          | 180                                               | -                                                 | -                                      | <b>E</b> in-plane               | "fused quartz"                                                         | [13]          |
|                                      | 330 nm          | 280                                               | -                                                 | 24                                     | (100) <sub>pc</sub>             | Si/SiO <sub>2</sub> /Ti/Pt                                             | [15]          |
|                                      | 330 nm          | 220                                               | -                                                 | 32                                     | (111) <sub>pc</sub>             | Si/SiO <sub>2</sub> /Ti/Pt/TiO <sub>2</sub>                            | [15]          |
| <b>Pulsed laser deposition (PLD)</b> |                 |                                                   |                                                   |                                        |                                 |                                                                        |               |
|                                      | -               | 150                                               | 80                                                | 44                                     | (122) <sub>o</sub>              | "platinum coated silicon"                                              | [16]          |
|                                      | 500 nm          | 156                                               | 84                                                | 36                                     | (110) <sub>pc</sub>             | "platinum-coated silicon"                                              | [17, 18]      |
|                                      | 390 nm          | 550                                               | 300                                               | 40                                     | (120) <sub>o</sub>              | SrTiO <sub>3</sub> /SrRuO <sub>3</sub>                                 | [19]          |
|                                      | 100 nm          | 700                                               | 300                                               | 40                                     | (001) <sub>o</sub>              | SrTiO <sub>3</sub> /BaZrO <sub>3</sub> /BaPbO <sub>3</sub>             | [19]          |
|                                      | 512 nm          | 661                                               | 400                                               | 20                                     | (100) <sub>pc</sub>             | Si/SiO <sub>2</sub> /Ti/Pt                                             | [6]           |
|                                      | 1000 nm         | 525                                               | 300                                               | 41                                     | (001) <sub>pc</sub>             | Si/Ca <sub>2</sub> Nb <sub>3</sub> O <sub>10</sub> /SrRuO <sub>3</sub> | [20]          |
| <b>Sputtering</b>                    |                 |                                                   |                                                   |                                        |                                 |                                                                        |               |
|                                      | 360 nm          | 630                                               | 365                                               | 31                                     | (001) <sub>pc</sub>             | Si/SiO <sub>2</sub> /LaNiO <sub>3</sub>                                | [21]          |
|                                      | 300 nm          | 380                                               | 200                                               | 21                                     | (001) <sub>pc</sub> , epitaxial | LaNiO <sub>3</sub> /SrTiO <sub>3</sub>                                 | [22]          |
|                                      | 300 nm          | 580                                               | 380                                               | 34                                     | (110) <sub>pc</sub> , epitaxial | LaNiO <sub>3</sub> /SrTiO <sub>3</sub>                                 | [22]          |
|                                      | 300 nm          | 500                                               | 320                                               | 36                                     | (111) <sub>pc</sub> , epitaxial | LaNiO <sub>3</sub> /SrTiO <sub>3</sub>                                 | [22]          |
|                                      | 3 $\mu\text{m}$ | 80                                                | 120                                               | 20                                     | Random                          | Si/SiO <sub>2</sub> /Ti/Pt                                             | [23]          |

- 
- [1] N. Godard, P. Grysan, E. Defay, and S. Glinšek, Growth of {100}-oriented lead zirconate titanate thin films mediated by a safe solvent, *Journal of Materials Chemistry C* (2020).
  - [2] B. Xu, Y. Ye, Q. M. Wang, and L. E. Cross, Dependence of electrical properties on film thickness in lanthanum-doped lead zirconate titanate stannate antiferroelectric thin films, *Journal of Applied Physics* **85**, 3753 (1999).
  - [3] T. Schenk, C. M. Fancher, M. H. Park, C. Richter, C. Künneth, A. Kersch, J. L. Jones, T. Mikolajick, and U. Schroeder, On the Origin of the Large Remanent Polarization in La:HfO<sub>2</sub>, *Advanced Electronic Materials* **5**, 1 (2019).
  - [4] X. G. Tang, J. Wang, X. X. Wang, and H. L. W. Chan, Electrical properties of highly (111)-oriented lead zirconate thin films, *Solid State Communications* **130**, 373 (2004).
  - [5] X. Hao, J. Zhai, J. Zhou, Z. Yue, J. Yang, W. Zhao, and S. An, Structure and electrical properties of PbZrO<sub>3</sub> antiferroelectric thin films doped with barium and strontium, *Journal of Alloys and Compounds* **509**, 271 (2011).
  - [6] M. D. Nguyen, T. T. Trinh, H. T. Dang, and H. N. Vu, Understanding the effects of electric-field-induced phase transition and polarization loop behavior on the energy storage performance of antiferroelectric PbZrO<sub>3</sub> thin films, *Thin Solid Films* **697**, 137794 (2020).
  - [7] X. Hao, J. Zhai, and X. Yao, Improved energy storage performance and fatigue endurance of Sr-Doped PbZrO<sub>3</sub> antiferroelectric thin films, *Journal of the American Ceramic Society* **92**, 1133 (2009).
  - [8] Z. Tang and X. Tang, Structural, dielectric and optical properties of highly oriented lead zirconate thin films prepared by sol-gel process, *Materials Chemistry and Physics* **80**, 294 (2003).
  - [9] J. Zhai and H. Chen, Direct current field and temperature dependent behaviors of antiferroelectric to ferroelectric switching in highly (100)-oriented PbZrO<sub>3</sub> thin films, *Applied Physics Letters* **82**, 2673 (2003).
  - [10] M. Guo, M. Wu, W. Gao, B. Sun, and X. Lou, Giant negative electrocaloric effect in antiferroelectric PbZrO<sub>3</sub> thin films in an ultra-low temperature range, *Journal of Materials Chemistry C* **7**, 617 (2019).
  - [11] M. Ye, Q. Sun, X. Chen, Z. Jiang, and F. Wang, Effect of Eu doping on the electrical properties and energy storage performance of PbZrO<sub>3</sub> antiferroelectric thin films, *Journal of the American Ceramic Society* **94**, 3234 (2011).
  - [12] J. Zhai, Y. Yao, X. Li, T. F. Hung, Z. K. Xu, H. Chen, E. V. Colla, and T. B. Wu, Dielectric properties of oriented PbZrO<sub>3</sub> thin films grown by sol-gel process, *Journal of Applied Physics* **92**, 3990 (2002).
  - [13] F. Wang, K. K. Li, and G. H. Haertling, Transverse electro-optic effect of antiferroelectric lead zirconate thin films, *Optics Letters* **17**, 1122 (1992).
  - [14] K. K. Li, F. Wang, and G. H. Haertling, Antiferroelectric lead zirconate thin films derived from acetate precursors, *Journal of Materials Science* **30**, 1386 (1995).
  - [15] T. Tani, J. F. Li, D. Viehland, and D. A. Payne, Antiferroelectric-ferroelectric switching and induced strains for sol-gel derived lead zirconate thin layers, *Journal of Applied Physics* **75**, 3017 (1994).
  - [16] S. S. N. Bharadwaja and S. B. Krupanidhi, Dielectric and dc electrical studies of antiferroelectric lead zirconate thin films, *Materials Science and Engineering B: Solid-State Materials for Advanced Technology* **B78**, 1 (2000).
  - [17] S. S. Bharadwaja and S. B. Krupanidhi, Growth and study of antiferroelectric lead zirconate thin films by pulsed laser ablation, *Journal of Applied Physics* **86**, 5862 (1999).
  - [18] P. S. Dobal, R. S. Katiyar, S. S. N. Bharadwaja, and S. B. Krupanidhi, Micro-Raman and dielectric phase transition studies in antiferroelectric PbZrO<sub>3</sub> thin films, *Applied Physics Letters* **78**, 1730 (2001).
  - [19] K. Boldyreva, D. Bao, G. Le Rhun, L. Pintilie, M. Alexe, and D. Hesse, Microstructure and electrical properties of (120)<sub>O</sub>-oriented and of (001)<sub>O</sub>-oriented epitaxial antiferroelectric PbZrO<sub>3</sub> thin films on (100) SrTiO<sub>3</sub> substrates covered with different oxide bottom electrodes, *Journal of Applied Physics* **102**, 044111 (2007).
  - [20] M. D. Nguyen and G. Rijnders, Electric field-induced phase transition and energy storage performance of highly-textured PbZrO<sub>3</sub> antiferroelectric films with a deposition temperature dependence, *Journal of the European Ceramic Society* **38**, 4953 (2018).
  - [21] X. Guo, J. Ge, F. Ponchel, D. Rémiens, Y. Chen, X. Dong, and G. Wang, Effect of Sn substitution on the energy storage properties of high (001)-oriented PbZrO<sub>3</sub> thin films, *Thin Solid Films* **632**, 93 (2017).
  - [22] J. Ge, D. Rémiens, X. Dong, Y. Chen, J. Costecalde, F. Gao, F. Cao, and G. Wang, Enhancement of energy storage in epitaxial PbZrO<sub>3</sub> antiferroelectric films using strain engineering, *Applied Physics Letters* **105**, 1 (2014).
  - [23] I. Kanno, T. Inoue, T. Suzuki, H. Kotera, and K. Wasa, Electric field-induced strain of PbZrO<sub>3</sub> films, *Japanese Journal of Applied Physics* **45**, 7258 (2006).
